# Supplementary material for: Sketched Adaptive Federated Deep Learning: A Sharp Convergence Analysis
Source: arXiv:2411.06770 source file (2025-04-13)
Supplement: Supplementary file 1 [file app_heavy_tail.tex]

\subsection{Proof of Lemma~\ref{descent_heavy_tail}}
\label{app_heavy}
Denote $\Delta_t^c = \sum_{k=1}^K g_{t,k}^c$, $\tilde{\Delta}_{t}^c = \min\{1, \frac{\tau}{\sumv{C}\Vert \Delta_t^c \Vert}\}\Delta_t^c$. Then $x_{t+1} - x_t = -\lr \eta R^\top R\sumv{C}\tilde{\Delta}_{t}^c$.
\begin{proof}
Taking the expectation of randomness in stochastic gradient yields
\begin{align*}
    &\E[\cL(x_{t+1})] - \cL(x_t)= -\lr \eta\langle \nabla \cL(x_t), \frac{1}{C} R^\top R \sum_{c=1}^C \E[\tilde{\Delta}_{t}^c] \rangle + \frac{\lr^2 \eta^2}{2} \E[(\frac{1}{C} R^\top R \sum_{c=1}^C \tilde{\Delta}_{t}^c)^\top \hat{H}_\cL (\frac{1}{C} R^\top R \sum_{c=1}^C \tilde{\Delta}_{t}^c)]\\
    &=  -\lr \eta\langle \nabla \cL(x_t), \frac{1}{C} \sum_{c=1}^C R^\top R \E[\tilde{\Delta}_{t}^c] - \E[\tilde{\Delta}_{t}^c]\rangle  -\lr \eta\langle \nabla \cL(x_t), \frac{1}{C} \sum_{c=1}^C \E[\tilde{\Delta}_{t}^c] \rangle \\
    &+ \frac{\lr^2 \eta^2}{2} \E[(\frac{1}{C} R^\top R \sum_{c=1}^C \tilde{\Delta}_{t}^c)^\top \hat{H}_\cL (\frac{1}{C} R^\top R \sum_{c=1}^C \tilde{\Delta}_{t}^c)]\\
    &\le \frac{\lr \eta K}{2} \logd\norm{\nabla \cL}^2 + \frac{\lr \eta}{2K} \logd \norm{\sumv{C} \E[\tdelta]}^2 -\frac{\lr \eta K}{2}\norm{\nabla \cL}^2 -\frac{\lr \eta }{2K} \norm{\sumv{C} \E[\tdelta]}^2 \\
    & + \frac{\lr \eta K}{2} \norm{\nabla \cL - \frac{1}{K} \sumv{C} \E[\tdelta]}^2 + \frac{\lr^2 \eta^2}{2} \E[(\frac{1}{C} R^\top R \sum_{c=1}^C \tilde{\Delta}_{t}^c)^\top \hat{H}_\cL (\frac{1}{C} R^\top R \sum_{c=1}^C \tilde{\Delta}_{t}^c)] \\
    &\le -(1-\logd) \frac{\lr \eta K}{2}\norm{\nabla \cL}^2 + \frac{\lr \eta K}{2} \norm{\nabla \cL - \frac{1}{K} \sumv{C} \E[\tdelta]}^2 \\
    &+ \frac{\lr^2 \eta^2}{2} \E[(\frac{1}{C} R^\top R \sum_{c=1}^C \tilde{\Delta}_{t}^c)^\top \hat{H}_\cL (\frac{1}{C} R^\top R \sum_{c=1}^C \tilde{\Delta}_{t}^c)]\\
    & \le - \frac{\lr \eta K}{4}\norm{\nabla \cL}^2 + \frac{\lr \eta K}{2} \norm{\nabla \cL - \frac{1}{K} \sumv{C} \E[\tdelta]}^2 \\
    & + \frac{\lr^2 \eta^2}{2} \E[(\frac{1}{C} R^\top R \sum_{i=1}^C \tilde{\Delta}_{t,i}^c)^\top \hat{H}_\cL (\frac{1}{C} R^\top R \sum_{i=1}^C \tilde{\Delta}_{t,i}^c)], ~~w.p.~ 1- \Theta(\delta)
\end{align*}
where the first inequality is directly from Lemma~\ref{lemma_srht}. The second and last inequalities are from the condition of $b \ge 4\log^3(d/\delta)$.
\end{proof}

\subsection{Proof of Theorem~\ref{theorem_heavy_tail}}
The first order term in Lemma~\ref{descent_heavy_tail} can be handled by
\begin{align*}
    &\norm{\nabla \cL - \frac{1}{K} \sumv{C} \E[\tdelta]} \le \norm{\nabla \cL - \frac{1}{K} \sumv{C} \E[\odelta]} + \frac{1}{K}\norm{\sumv{C} \E[\odelta] - \sumv{C}\E[\tdelta]} \\
    &\le \frac{\eta L}{KC} \sum_{c=1}^C \sum_{i=1}^K \E[\norm{\nabla \cL_{t,k}^c}] + \frac{1}{KC} \sum_{c=1}^C \E[\norm{\odelta} 1_{\{\sumv{C} \norm{\odelta} \ge \tau \}}]\\
    &\le \eta K LG + K^{\alpha-1} G^\alpha \tau^{1-\alpha},
\end{align*}
where the last inequality follows by 
\begin{comment}
    \begin{align*}
    &\sum_{c=1}^C \E[\norm{\odelta} 1_{\{\sumv{C} \norm{\odelta} \ge \tau \}}] = (\sum_{c=1}^C \E[\norm{\odelta} 1_{\{\sumv{C} \norm{\odelta} \ge \tau \}}] )^\alpha (\E[\sum_{c=1}^C \norm{\odelta} 1_{\{\sumv{C} \norm{\odelta} \ge \tau \}}] )^{1-\alpha} \\
    &\le (\sum_{c=1}^C \E[\norm{\odelta}])^\alpha (\E[\sum_{c=1}^C \norm{\odelta} 1_{\{\sumv{C} \norm{\odelta} \ge \tau \}}] )^{1-\alpha} \le C(KG)^\alpha \tau^{1-\alpha}.
\end{align*}
\end{comment}
\begin{align*}
    &\frac{1}{C}\sum_{c=1}^C \E[\norm{\odelta} 1_{\{\sumv{C} \norm{\odelta} \ge \tau \}}] = \E[\sumv{C}\norm{\odelta} 1_{\{\sumv{C} \norm{\odelta} \ge \tau \}}] \\
    &=\E[(\sumv{C}\norm{\odelta})^{\alpha} (\sumv{C}\norm{\odelta})^{1-\alpha} 1_{\{\sumv{C} \norm{\odelta} \ge \tau \}}] \le (KG)^\alpha \tau^{1-\alpha}.
\end{align*}

The second order term can be handled as follows.
With probability $1-\Theta(\delta)$,
\begin{align*}
    &\E[(\frac{1}{C} R^\top R \sum_{i=1}^C \tilde{\Delta}_{t,i}^c)^\top \hat{H}_\cL (\frac{1}{C} R^\top R \sum_{i=1}^C \tilde{\Delta}_{t,i}^c)] = \E[\sum_{j=1}^d \lambda_j \langle \frac{1}{C} R^\top R \sum_{i=1}^C \tilde{\Delta}_{t,i}^c , v_j\rangle^2] \\
    &\le \E[\sum_{j=1}^d  \lambda_j 1_{\lambda_j  \ge 0} \langle \frac{1}{C} R^\top R \sum_{i=1}^C \tilde{\Delta}_{t,i}^c , v_j\rangle^{2-\alpha} \langle \frac{1}{C} R^\top R \sum_{i=1}^C \tilde{\Delta}_{t,i}^c , v_j\rangle^{\alpha}] \\
    &\le \E\left[\sum_{j=1}^d  \lambda_j 1_{\lambda_j  \ge 0} \left((1+\logd) \frac{\tau}{\sumv{C} \norm{\odelta} } \sumv{C} \norm{\odelta} \right)^{2-\alpha} \left(\frac{1}{C} (1+\logd) \sum_{i=1}^C \norm{\odelta}\right)^{\alpha}\right] \\
    & \le (1+\logd)\sumL K^2 \tau^{2-\alpha}G^\alpha,
\end{align*}
where the first equation follows by using the eigen-decomposition of $\hat H_\cL$ and the second order term can be reduced to a squared inner product term. The primary trick thereafter (in the first inequality) is to split the inner product terms into two parts, which can be handled by the two-sided adaptive learning rates respectively. By applying the bounded second moment of random sketching, we find the first part with order $2-\alpha$ is contained in a $(1+\logd)\tau-$ball with high probability, and the second part with order $\alpha$ is bounded by applying Assumption~\ref{assume_heavy_tail}. Then Theorem~\ref{theorem_heavy_tail} follows by combining the first order term and the second-order term by union bounds, as well as applying the condition of $b \ge 4\log^3(d/\delta)$.
