# Supplementary material for: Sketched Adaptive Federated Deep Learning: A Sharp Convergence Analysis
Source: arXiv:2411.06770 source file (2025-04-13)
Supplement: Supplementary file 2 [file app_discussion.tex]

\subsection{Limitations}
In this work, we do not cover all the potential benefits of random sketching, e.g. privacy. We also do not account for the degrade in generalization performance when the compression rate is low.

\subsection{Broader Impacts}
This work will facilitate distributed learning in achieving higher communication efficiency. But the wide usage of distirbuted training may also incur malicious attacks and data poisioning to the federated system.
