# Supplementary material for: Sketched Adaptive Federated Deep Learning: A Sharp Convergence Analysis
Source: arXiv:2411.06770 source file (2025-04-13)
Supplement: Supplementary file 3 [file app_variant_optimizers.tex]

\begin{algorithm}[t]
  \caption{AMS\_Step}
  \SetAlgoLined
  \KwData{Learning rate $\lr$, $\beta_1$, $\beta_2$, Small constant $\epsilon$, iterate $x_t$, sketched moments $\bar{m}_t$, $\bar{v}_t$}\\
  \KwResult{Updated parameters $\x_{t+1}$}
  Initialize $m_0 = 0$, $v_0 = 0$, $\hat{v}_0 = 0$\;
    Update first moment estimate:~~ $m_t = \beta_1 \cdot m_{t-1} + (1 - \beta_1) \cdot \decomp(\bar{m}_t).$;
    
    Update second moment estimate:~~ $v_t = \beta_2 \cdot v_{t-1} + (1 - \beta_2) \cdot \decomp(\bar{v}_t)$;
    
    Update maximum of past second moment estimates: 
    $\hat{v}_t = \max(\hat{v}_{t-1}, v_t).$
    
    Update parameters:
    $x_{t+1} = x_{t} - \frac{\lr}{\sqrt{\hat{v}_t} + \epsilon} \cdot m_t := x_t - \kappa {\hat{V}_{t}}^{-1/2} m_t$.
  %}
  \label{alg:ams}
%\vspace*{-3mm}
\end{algorithm}
